# Supplementary material for: LibppRPA: An Open-Source Library for Particle-Particle Random Phase Approximation
Source: arXiv:2512.12515 ancillary file (2025-12-14)
Supplement: Supplementary file 1 [file supporting_information.pdf]

# Supporting Information: LibppRPA: An Open-Source Library for Particle-Particle Random Phase Approximation

Jincheng Yu,[†] Jiachen Li,[¶] Chaoqun Zhang,[¶] Tianyu Zhu,[¶] and Weitao Yang[*,†]

†*Department of Chemistry, Duke University, Durham, North Carolina 27708, United States*

‡*Department of Chemistry and Biochemistry, University of Maryland, College Park, Maryland 20742, United States*

¶*Department of Chemistry, Yale University, New Haven, Connecticut 06520, United States*

E-mail: weitao.yang@duke.edu

# 1 Singlet-Triplet Gaps of Diradicals

Table S1: Mean absolute errors (MAEs) of singlet-triplet gaps of diradicals obtained from ppRPA and SF-TDDFT based on HF, PBE and B3LYP. SF-TDDFT results were taken from Ref. S1. Geometries were taken from Refs. S2,S3. Reference values were taken from Refs. S1,S4. The aug-cc-pVTZ basis set was used. All values are in kcal/mol.

| | HF | PBE | B3LYP |
|---|---|---|---|
| ppRPA | 17.5 | 3.9 | 4.7 |
| SF-TDDFT | | 27.2 | 25.8 |

To properly describe diradical systems, ppRPA starts with the $(N-2)$-electron system and then adds two electrons with explicit correlation. The closed-shell $(N-2)$-electron system can be well described by a single-determinant DFT reference, which makes ppRPA free of the spin contamination. Because of the seamless combination of a subspace configuration interaction fashion for two diradical electrons and DFT for the remaining $(N-2)$ electrons, ppRPA is almost free from the static correlation error and provides accurate predictions of singlet-triplet gaps of diradical systems. Table S1 presents the mean absolute errors (MAEs) of ppRPA in predicting vertical and adiabatic singlet-triplet gaps across various categories of diradicals, including diatomic, carbene-like, disjoint, and four-$\pi$-electron diradicals. It shows that SF-TDDFT gives large errors of 25 kcal/mol to predict accurate singlet-triplet gaps of diradicals. ppRPA based on two DFT references significantly outperforms SF-TDDFT with errors only around 4 kcal/mol. The starting point dependence in ppRPA is smaller than that in SF-TDDFT. The difference between ppRPA@PBE and ppRPA@B3LYP is less than 1 kcal/mol. As shown in Ref. S5, the multireference character of diradical systems can be quantified with ppRPA by analyzing the dominant configuration contributions.

Table S2: Singlet-triplet gaps of diradicals obtained from ppRPA based on HF, PBE and B3LYP. Geometries were taken from Refs. S2,S3. Reference values were taken from Refs. S1,S4. The aug-cc-pVTZ basis set was used. All values are in kcal/mol.

| | | | ref | ppRPA@HF | ppRPA@PBE | ppRPA@B3LYP |
|---|---|---|---|---|---|---|
| $\cdot CH_2CH_2CH_2\cdot$ | vertical | | 1.8 | 0.0 | 0.0 | 0.0 |
| $\cdot CH_2(CH_2)_4CH_2\cdot$ | vertical | $^1A_1$ | 0.0 | 0.0 | 0.0 | 0.0 |
| | vertical | $^1B_1$ | 160.8 | 79.4 | 159.4 | 147.6 |
| | vertical | $2^1A_1$ | 163.1 | 80.1 | 162.1 | 149.2 |
| $\cdot CH_2(CH_2)_4C(CH_3)H\cdot$ | vertical | $^1A_1$ | -0.2 | 0.0 | 0.0 | 0.0 |
| | vertical | $2^1A_1$ | 131.1 | 65.5 | 140.0 | 129.3 |
| | vertical | $3^1A_1$ | 144.3 | 77.3 | 152.5 | 142.3 |
| cyclobutadiene | vertical | | 7.2 | 0.0 | 0.0 | 0.0 |
| NH | adiabatic | | 35.9 | 29.4 | 38.2 | 36.3 |
| $OH^+$ | adiabatic | | 50.5 | 44.1 | 51.7 | 50.0 |
| NF | adiabatic | | 34.3 | 27.2 | 27.0 | 27.2 |
| $O_2$ | adiabatic | | 22.6 | 22.6 | 22.9 | 22.9 |
| $CH_2$ | adiabatic | $^1A_1$ | 9.7 | -3.6 | 4.9 | 2.6 |
| | adiabatic | $^1B_1$ | 32.5 | 25.5 | 31.7 | 30.4 |
| | adiabatic | $2^1A_1$ | 58.3 | 47.6 | 53.3 | 51.7 |
| $NH_2{}^+$ | adiabatic | $^1A_1$ | 28.9 | 9.8 | 23.8 | 21.0 |
| | adiabatic | $^1B_1$ | 43.0 | 35.8 | 41.4 | 39.9 |
| | adiabatic | $2^1A_1$ | 76.5 | 62.5 | 69.6 | 67.8 |
| $SiH_2$ | adiabatic | $^1A_1$ | -20.6 | -26.0 | -29.6 | -29.9 |
| | adiabatic | $^1B_1$ | 24.1 | 23.2 | 25.0 | 25.0 |
| | adiabatic | $2^1A_1$ | 57.0 | 52.8 | 51.7 | 53.1 |
| $PH_2{}^+$ | adiabatic | $^1A_1$ | -18.3 | -26.5 | -25.0 | -26.0 |
| | adiabatic | $^1B_1$ | 27.6 | 27.8 | 28.4 | 28.5 |

Table S2: Continued

| | | ref | ppRPA@HF | ppRPA@PBE | ppRPA@B3LYP |
|---|---|---|---|---|---|
| adiabatic | $2^1A_1$ | 65.6 | 62.2 | 58.0 | 59.8 |

# 2 Double Excitation Energies of Molecules

Table S3: Mean absolute errors (MAEs) of double excitation energies of molecular systems obtained from ppRPA based on different functionals. Results of ppRPA were taken from Ref. S6 and of wave function approaches were taken from Ref. S7. Reference values were taken from Ref. S7. The aug-cc-pVTZ basis set was used. All values are in eV.

| ppRPA | MAE | wave function | MAE |
|---|---|---|---|
| B3LYP | 0.39 | CCSDTQ | 0.03 |
| M06-2X | 0.60 | CC4 | 0.05 |
| TPSSh | 0.36 | CCSDT | 0.28 |
| PBE | 0.38 | CC3 | 0.56 |
| SCAN | 0.44 | SA-CASSCF | 0.48 |
| CAM-B3LYP | 0.52 | CASPT2 | 0.23 |
| HSE03 | 0.43 | | |
| $\omega$B97X-D | 0.53 | | |

Compared to particle-hole formalisms, one of the major advantages of ppRPA is that it incorporates two-particle information from the particle-particle and hole-hole channels, which makes it naturally adept at describing double excitations. MAEs of ppRPA based on different functionals for predicting double excitation energies of molecular systems are shown in Table S3. For ppRPA starting with GGA functionals, the HOMO and LUMO energy of the $(N-2)$-electron system can be degenerate, which leads to difficulties in the SCF convergence. Thus, hybrid functionals are the better starting point for ppRPA to describe double excitations. Fortunately, highly degenerate cases are rare, particularly in large molecules. It shows ppRPA based on exchange-correlation functionals with appropriate amounts of HF ex-

change provides accuracy comparable to high-level wave function methods. ppRPA based on B3LYP and TPSSh gives MAEs only around 0.4 eV, close to the computationally demanding CCSDT approach. in the ppRPA@B3LYP calculation for acrolein As demonstrated in Ref. S6, NTO weights obtained from ppRPA provides a tool to characterize genuine or partial nature of double excitations, which agrees with the description by wave function approaches.

# 3 Charge-Transfer Excitation Energies of Stein Set

Table S4: Mean absolute errors (MAEs) of charge-transfer excitation energies in Stein set obtained from ppRPA, TDDFT and BSE/$G_0W_0$ based on HF, PBE and B3LYP. TDDFT and BSE/$G_0W_0$ results were taken from Ref. S8. Geometries were taken from Ref. S9. Experiment values in the gas phase were taken as the reference values.[S9] Gas phase experimental references were used. The cc-pVDZ basis set was used. All values are in eV.

| | HF | PBE | B3LYP |
|---|---|---|---|
| ppRPA | 0.51 | 0.86 | 0.72 |
| TDDFT | 0.78 | 1.45 | 1.16 |
| BSE/$G_0W_0$ | 0.10 | 1.31 | 0.74 |

Because the ppRPA kernel provides the correct long-range asymptotic behavior, ppRPA is capable of predicting accurate charge transfer excitation energies. The MAEs of ppRPA, TDDFT and BSE/$G_0W_0$ for predicting 12 intramolecular charge transfer excitations between an aromatic donor and the tetracyanoethylene acceptor in Stein's set[S9] are shown in Table S4. TDDFT with GGA functional fails to predict charge transfer excitations with errors around 1.5 eV. MAEs of TDDFT largely reduce with increased percentage of HF exchange. Because of the dynamical screening and the correct long-range behavior, BSE/$G_0W_0$ based on DFT references provides improvements about 0.1 to 0.4 eV over TDDFT. BSE/$G_0W_0$@HF provides the smallest MAE of 0.1 eV due to the error cancellation. ppRPA outperforms TDDFT for all starting points with MAEs reduced by 0.3 to 0.6 eV. Because asymptotic trend is independent of any functional references, ppRPA also shows the smallest starting point dependence among three approaches. The difference between ppRPA@HF and

ppRPA@PBE is only around 0.3 eV.

Table S5: Charge-transfer excitation energies in Stein charge-transfer set obtained from ppRPA based on HF, PBE and B3LYP. Geometries and reference values were taken from Ref. S9. The cc-pVDZ basis set was used. All values are in eV.

| | ref(liquid) | ref(gas) | HF | PBE | B3LYP |
|---|---|---|---|---|---|
| anthracene | 1.73 | 2.05 | 1.96 | | 1.36 |
| 9-cyano | 2.01 | 2.33 | 2.00 | 1.36 | 1.49 |
| 9-cholo | 1.74 | 2.06 | 1.92 | 1.20 | 1.32 |
| 9-carbo-methoxy | 1.84 | 2.16 | 1.92 | 1.19 | 1.30 |
| 9-methyl | 1.55 | 1.87 | 1.71 | 1.06 | 1.16 |
| 9,10-dimethyl | 1.44 | 1.76 | 1.79 | 1.07 | 1.20 |
| 9-formyl | 1.90 | 2.22 | 2.09 | | 1.51 |
| 9-formyl, 10-chloro | 1.96 | 2.28 | 2.14 | | 1.52 |
| benzene | 3.59 | 3.91 | 2.69 | | 3.46 |
| toluene | 3.36 | 3.68 | 2.31 | | 2.99 |
| o-xylene | 3.15 | 3.47 | 1.85 | | 2.61 |
| naphthalene | 2.60 | 2.92 | 2.24 | | 2.18 |

# 4 Rydberg Excitation Energies of Small Atomic and Molecular Systems

The MAEs of ppRPA, TDDFT and BSE/$G_0W_0$ for predicting Rydberg excitations of atomic systems are shown in Table S6. It shows that TDDFT gives large MAEs for all starting points. BSE/$G_0W_0$ provides slight improvement for DFT references and significantly outperforms TDDFT for the HF reference. ppRPA based on the HF reference provides the smallest MAE of only 0.08 eV. However, ppRPA based on DFT references gives MAEs larger

Table S6: Mean absolute errors (MAEs) of Rydberg excitation energies of atomic systems obtained from ppRPA, TDDFT and BSE/$G_0W_0$ based on HF, PBE and B3LYP. TDDFT and BSE/$G_0W_0$ results were taken from Ref. S10. Reference values were taken from Ref. S11. The aug-cc-pVQZ basis set was used. All values are in eV.

| | HF | PBE | B3LYP |
|---|---|---|---|
| ppRPA | 0.08 | 2.13 | 2.53 |
| TDDFT | 0.92 | 1.03 | 0.86 |
| BSE/$G_0W_0$ | 0.16 | 0.97 | 0.73 |

than 2 eV.

Table S7: Rydberg excitation energies of atomic systems obtained from ppRPA, TDDFT and BSE/$G_0W_0$ based on HF, PBE and B3LYP. TDDFT and BSE/$G_0W_0$ results were taken from Ref. S10. Reference values were taken from Ref. S11. The aug-cc-pVQZ basis set was used. All values are in eV.

| | state | ref | HF | PBE | B3LYP |
|---|---|---|---|---|---|
| Be | triplet 2s→3s | 6.46 | 6.47 | 7.96 | 8.37 |
| | singlet 2s→3s | 6.78 | 6.79 | 8.26 | 8.66 |
| $B^+$ | triplet 2s→3s | 16.09 | 16.07 | 18.59 | 19.45 |
| | singlet 2s→3s | 17.06 | 17.09 | 19.41 | 20.25 |
| Mg | triplet 3s→4s | 5.11 | 5.01 | 7.05 | 7.16 |
| | singlet 3s→4s | 5.39 | 5.30 | 7.31 | 7.42 |
| $Al^+$ | triplet 3s→4s | 11.32 | 11.15 | 14.02 | 14.26 |
| | singlet 3s→4s | 11.82 | 11.64 | 14.50 | 14.72 |

# 5 Excitation Energies of Thiel Set

Table S8: Mean absolute errors (MAEs) of excitation energies in Thiel's set obtained from ppRPA and TDDFT based on HF, PBE and B3LYP. TDDFT results were taken from Ref. S12. Geometries and reference values were taken from Ref. S13. The aug-cc-pVDZ basis set was used. All values are in eV.

| | HF | PBE | B3LYP |
|---|---|---|---|
| ppRPA | 0.79 | 0.39 | 0.37 |
| TDDFT | 1.82 | 0.37 | 0.49 |

eV. For the HF reference, the MAE of ppRPA is much smaller than that of TDDFT. Because the ppRPA kernel is independent of the DFT reference, the difference between ppRPA based on GGA and hybrid functionals is less than 0.05 eV, which is much smaller than that in TDDFT. In the ppRPA calculations for valence excitations, excitations with incorrect symmetry are found below the desired excitations in many cases, especially in ppRPA@HF. This excitation misalignment also happens sometimes in TDHF or CIS calculations.[S12]

Table S9: Excitation energies in Thiel set obtained from ppRPA based on HF, PBE and B3LYP. Geometries and reference values were taken from Ref. S13. The aug-cc-pVDZ basis set was used. All values are in eV.

| | state | ref | HF | PBE | B3LYP |
|---|---|---|---|---|---|
| ethene | $^3B_{1u}$ | 4.50 | 3.93 | 3.48 | 3.62 |
| ethene | $^1B_{1u}$ | 7.80 | 6.26 | 8.86 | 8.46 |
| butadiene | $^3B_u$ | 3.20 | 3.22 | 2.28 | 2.52 |
| butadiene | $^3A_g$ | 5.08 | 5.60 | 5.85 | 6.07 |
| butadiene | $^1B_u$ | 6.18 | 5.49 | 6.51 | 6.57 |
| butadiene | $^1A_g$ | 6.55 | 5.92 | 6.11 | 6.44 |
| hexatriene | $^3B_u$ | 2.40 | 2.59 | 1.61 | 1.88 |
| hexatriene | $^3A_g$ | 4.15 | 5.21 | 4.47 | 4.86 |
| hexatriene | $^1A_g$ | 5.09 | 5.42 | 4.49 | 4.99 |
| hexatriene | $^1B_u$ | 5.10 | 5.04 | 5.13 | 5.29 |
| octetraene | $^3B_u$ | 2.20 | 2.15 | 1.21 | 1.49 |
| octetraene | $^3A_g$ | 3.55 | 4.75 | 3.57 | 4.00 |
| octetraene | $^1A_g$ | 4.47 | 5.02 | 3.53 | 4.08 |
| octetraene | $^1B_u$ | 4.66 | 4.58 | 4.29 | 4.50 |
| cyclopropene | $^3B_2$ | 4.34 | 4.22 | 3.91 | 4.08 |
| cyclopropene | $^1B_2$ | 7.06 | 5.87 | 7.31 | 7.30 |
| cyclopentadiene | $^3B_2$ | 3.25 | 3.12 | 2.53 | 2.66 |

Table S9: Continued

| | state | ref | HF | PBE | B3LYP |
|---|---|---|---|---|---|
| cyclopentadiene | $^3A_1$ | 5.09 | 5.45 | 5.07 | 5.33 |
| cyclopentadiene | $^1B_2$ | 5.55 | 5.16 | 5.45 | 5.47 |
| cyclopentadiene | $^1A_1$ | 6.31 | 6.01 | 6.16 | 6.42 |
| norbornadiene | $^3A_2$ | 3.72 | 3.77 | 3.58 | 3.69 |
| norbornadiene | $^3B_2$ | 4.16 | 4.49 | 4.51 | 4.76 |
| norbornadiene | $^1A_2$ | 5.34 | 3.96 | 5.35 | 5.36 |
| norbornadiene | $^1B_2$ | 6.11 | 4.59 | 7.00 | 6.79 |
| furan | $^3B_2$ | 4.17 | 3.82 | 3.37 | 3.49 |
| furan | $^3A_1$ | 5.48 | 5.79 | 5.12 | 5.38 |
| furan | $^1B_2$ | 6.32 | 5.09 | 6.58 | 6.51 |
| furan | $^1A_1$ | 6.57 | 6.61 | 6.66 | 6.88 |
| s-tetrazine | $^3B_{3u}$ | 1.89 | 3.28 | 1.87 | 2.19 |
| s-tetrazine | $^3A_u$ | 3.52 | 5.38 | 3.16 | 3.67 |
| s-tetrazine | $^1B_{3u}$ | 2.24 | 3.78 | 2.41 | 2.73 |
| s-tetrazine | $^1A_u$ | 3.48 | 5.60 | 3.40 | 3.91 |
| formaldehyde | $^3A_2$ | 3.50 | 1.65 | 3.39 | 3.14 |
| formaldehyde | $^1A_2$ | 3.88 | 2.00 | 3.96 | 3.68 |
| acetone | $^3A_2$ | 4.05 | 3.10 | 4.24 | 4.13 |
| acetone | $^1A_2$ | 4.40 | 3.38 | 4.66 | 4.55 |
| benzoquinone | $^3B_{1g}$ | 2.51 | 3.15 | 2.44 | 2.93 |
| benzoquinone | $^1B_{1g}$ | 2.78 | 4.16 | 2.65 | 3.14 |

Table S10: Mean absolute errors (MAEs) of excitation energies of point defects obtained from ppRPA and TDDFT based on PBE and B3LYP. Results were taken from Refs. S14,S15. The cc-pVDZ basis set was used for ppRPA. All values are in eV.

| | PBE | B3LYP |
|---|---|---|
| ppRPA | 0.20 | 0.12 |
| TDDFT | 0.52 | 0.35 |

# 6 Excitation Energies of Point Defects

In this section, we demonstrate the applicability of ppRPA for calculating excitation energies of periodic systems. As shown in Refs. S14,S15, the corresponding ($N \pm 2$)-electron system of a broad range of point defects closed-shell, which can be well described by the single-reference DFT method. Then all desired defect states can be accessed on the equal footing by adding/removing two electrons. MAEs of vertical excitation energies of point defects obtained from ppRPA and TDDFT based on PBE and B3LYP are shown in Table S10. It shows that ppRPA based on both GGA and hybrid functionals significantly outperforms TDDFT with MAEs around 0.15 eV. The starting point dependence in ppRPA is largely reduced compared to TDDFT. In particular, ppRPA achieves good accuracy for excitation energies of point defects whose ground state has a strong multireference character, which is challenging for single-reference methods such as TDDFT and BSE/$GW$. Furthermore, as demonstrated in Ref. S15 the NTO approach in ppRPA provides important physical insights into electronic transitions in defect systems and the multireference character of associated states. Thus, ppRPA is an accurate and low-cost tool for investigating the excited-state properties of point defect systems.

Table S11: Excitation energies of point defects obtained from ppRPA and TDDFT based on PBE and B3LYP. The cc-pVDZ basis set was used for ppRPA. All values are in eV.

| | | | ppRPA | | TDDFT | |
|---|---|---|---|---|---|---|
| | state | ref | PBE | B3LYP | PBE | B3LYP |
| $NV^-$ in diamond | $^1E$ | 0.50∼0.59 | 0.53 | 0.61 | 0.51 | 0.69 |
| | $^1A_1$ | 1.76∼1.85 | 1.67 | 1.97 | 1.34 | 2.12 |
| | $^3E$ | 2.18 | 1.95 | 2.10 | 2.09 | 2.39 |
| $SiV^0$ in diamond | $^3A_{2u}$ | | 1.27 | 1.41 | 1.24 | 1.41 |
| | $^3E_u$ | 1.57 | 1.30 | 1.50 | 1.28 | 1.50 |
| | $^3A_{1u}$ | | 1.54 | 1.81 | 1.37 | 1.81 |
| $VV^0$ in 4H-SiC | $^1E$ | | 0.28 | 0.26 | 0.33 | 0.43 |
| | $^1A_1$ | | 0.88 | 0.80 | 0.90 | 1.58 |
| | $^3E$ | 1.24 | 1.12 | 0.88 | 1.41 | 1.45 |
| VC in diamond ($D_{2d}$) | $^1E$ | 2.2 | 1.77 | 2.15 | 1.26 | 1.40 |
| VC in diamond ($T_d$) | $1T_2$ | | 1.56 | 1.89 | | |
| VO in MgO | $^1T_{1u}$ | 5.0 | 4.82 | 5.05 | 3.37 | 4.29 |
| | $^3T_{1u}$ | 2.3∼2.4 | 3.57 | 3.58 | 3.08 | 3.42 |

In TableS11, ppRPA and TDDFT results were taken from Refs S14,S15. Experiment values for the nitrogen-vacancy ($NV^-$) in diamond were taken from Ref. S16,S17, for silicon-vacancy ($SiV^0$) in diamond were taken from Ref. S14, for divacancy center ($VV^0$) in 4H silicon carbide (4H-SiC) were taken from Ref. S14, for carbon-vacancy (VC) in diamond were taken from Ref. S18 for oxygen-vacancy (VO) in magnesium oxide (MgO) were taken from Ref. S19,S20. In calculation for mean absolute errors (MAEs), for the $^1E$ state and the $^1A_1$ state of $NV^-$ in diamond and the $^1T_{1u}$ state of VO in MgO, the average between the upper and the lower limits were used. The $^3T_{1u}$ state of VO in MgO was not included in MAE calculations, because the experimental measurement was conducted for the emission

process.

## 7 Reaction Barriers in DBH24 Set

Table S12: Mean absolute errors (MAEs) of reaction barriers in DBH24 set and its four subsets obtained from phRPA and ppRPA based on HF, PBE and B3LYP. Geometries and references were taken from Ref. S21. The aug-cc-pVDZ basis set was used. All values are in kcal/mol.

| | phRPA | | | ppRPA | | |
|---|---|---|---|---|---|---|
| | HF | PBE | B3LYP | HF | PBE | B3LYP |
| HAT | 12.01 | 3.71 | 3.54 | 10.45 | 5.80 | 4.90 |
| NS | 1.70 | 3.98 | 2.87 | 1.42 | 3.67 | 2.84 |
| UA | 4.65 | 1.49 | 1.38 | 3.51 | 1.60 | 1.54 |
| HT | 5.26 | 2.11 | 1.49 | 4.51 | 2.71 | 2.14 |
| total | 5.90 | 2.82 | 2.32 | 4.97 | 3.44 | 2.85 |

MAEs of reaction barriers of DBH24 set obtained from ppRPA and phRPA based on HF, PBE and B3LYP are shown in Table S12. Our results agree well with the literature results in Ref. S22. For four different types of reactions including hydrogen-transfer (HT), heavy-atom transfer (HAT), nucleophilic substitution (NS) and unimolecular and association (UA), ppRPA shows a similar accuracy to phRPA. Both ppRPA and phRPA based on DFT references provide smaller MAEs around 3 kcal/mol than those around 5 kcal/mol based on the HF reference. As discussed in Ref. S23, pp-RPA generally slightly underestimates absolute correlation energies and describes thermodynamic properties well, which suggests that the pp-RPA gives reliable energies in chemical applications.

Table S13: Reaction barriers in DBH24 set and its four subsets obtained from phRPA based on HF, PBE and B3LYP. f means forward, b means backward. Geometries and references were taken from Ref. S21. The aug-cc-pVDZ basis set was used. All values are in kcal/mol.

| | | phRPA@HF | | phRPA@PBE | | phRPA@B3LYP | |
|---|---|---|---|---|---|---|---|
| | | f | b | f | b | f | b |
| HAT | $H+N_2O \rightarrow OH+N_2$ | 31.16 | 101.73 | 15.65 | 86.83 | 17.76 | 86.99 |
| | $H+ClH \rightarrow HCl+H$ | 29.14 | 29.14 | 20.38 | 20.38 | 21.52 | 21.52 |
| | $CH_3+FCl \rightarrow CH_3F+Cl$ | 13.11 | 73.57 | -1.46 | 58.51 | 0.55 | 57.86 |
| NS | $Cl^-...CH_3Cl \rightarrow ClCH3...Cl^-$ | 14.45 | 14.45 | 9.34 | 9.34 | 10.51 | 10.51 |
| | $F^-...CH_3Cl \rightarrow FCH_3...Cl^-$ | 3.56 | 32.91 | 0.11 | 25.55 | 1.13 | 26.95 |
| | $OH^-+CH_3F \rightarrow HOCH_3+F^-$ | -1.64 | 20.77 | -7.15 | 13.19 | -6.49 | 14.48 |
| UA | $H+N_2 \rightarrow HN_2$ | 25.91 | 11.96 | 14.86 | 10.49 | 15.93 | 11.04 |
| | $H+C_2H_4 \rightarrow CH_3CH_2$ | 9.95 | 47.14 | 3.18 | 41.08 | 3.58 | 42.28 |
| | $HCN \rightarrow HNC$ | 48.14 | 34.89 | 44.34 | 30.52 | 45.40 | 31.53 |
| HT | $OH+CH_4 \rightarrow CH_3+H_2O$ | 13.35 | 22.32 | 7.37 | 14.34 | 7.15 | 15.93 |
| | $H+OH \rightarrow O+H_2$ | 17.68 | 19.90 | 8.09 | 14.66 | 9.36 | 14.57 |
| | $H+H_2S \rightarrow H_2+HS$ | 9.92 | 19.40 | 3.61 | 19.86 | 4.45 | 18.45 |

Table S14: Reaction barriers in DBH24 set and its four subsets obtained from ppRPA based on HF, PBE and B3LYP. f means forward, b means backward. Geometries and references were taken from Ref. S21. The aug-cc-pVDZ basis set was used. All values are in kcal/mol.

| | | ppRPA@HF | | ppRPA@PBE | | ppRPA@B3LYP | |
|---|---|---|---|---|---|---|---|
| | | f | b | f | b | f | b |
| HAT | $H+N_2O \rightarrow OH+N_2$ | 30.33 | 97.25 | 22.19 | 71.43 | 23.12 | 76.34 |
| | $H+ClH \rightarrow HCl+H$ | 26.78 | 26.78 | 23.42 | 23.42 | 24.08 | 24.08 |
| | $CH_3+FCl \rightarrow CH_3F+Cl$ | 12.83 | 74.53 | 1.16 | 59.18 | 2.42 | 61.38 |

Table S14: Continued

| | | ppRPA@HF | | ppRPA@PBE | | ppRPA@B3LYP | |
|---|---|---|---|---|---|---|---|
| | | f | b | f | b | f | b |
| NS | $Cl^-$...$CH_3Cl$→ClCH3...$Cl^-$ | 14.13 | 14.13 | 10.88 | 10.88 | 11.33 | 11.33 |
| | $F^-$...$CH_3Cl$→$FCH_3$...$Cl^-$ | 3.30 | 32.60 | 1.09 | 25.21 | 1.59 | 26.42 |
| | $OH^-$+$CH_3F$→$HOCH_3$+$F^-$ | -2.22 | 20.89 | -9.01 | 13.24 | -7.90 | 14.48 |
| UA | H+$N_2$→$HN_2$ | 23.43 | 11.33 | 17.89 | 10.42 | 18.44 | 10.77 |
| | H+$C_2H_4$→$CH_3CH_2$ | 6.36 | 45.67 | 4.56 | 42.48 | 4.76 | 42.82 |
| | HCN→HNC | 49.12 | 35.31 | 47.55 | 31.20 | 47.84 | 32.11 |
| HT | OH+$CH_4$→$CH_3$+$H_2O$ | 12.00 | 24.49 | 1.58 | 17.91 | 3.58 | 18.86 |
| | H+OH→O+$H_2$ | 17.04 | 19.17 | 14.43 | 12.25 | 14.69 | 13.50 |
| | H+$H_2S$→$H_2$+HS | 7.46 | 17.88 | 6.28 | 15.10 | 6.68 | 15.78 |

# 8 Dissociation Curves of $H_2$ and $Ar_2$

Table S15: Total energies of $H_2$ obtained from HF, phRPA@HF, ppRPA@HF, multireference DFT ppRPA@HF and CCSD. The cc-pVDZ basis set was used. All bond lengths are in angstrom and energy values are in Hartree.

| bond length | HF | phRPA@HF | ppRPA@HF | MR-ppRPA@HF | CCSD |
|---|---|---|---|---|---|
| 0.5 | -0.286760 | -0.193430 | -0.235610 | -0.080890 | -0.080810 |
| 0.6 | -0.344850 | -0.252990 | -0.294210 | -0.140710 | -0.140610 |
| 0.7 | -0.364880 | -0.274220 | -0.314630 | -0.162450 | -0.162340 |
| 0.8 | -0.364960 | -0.275250 | -0.314990 | -0.164310 | -0.164190 |
| 0.9 | -0.354350 | -0.265440 | -0.304600 | -0.155650 | -0.155520 |
| 1.0 | -0.338110 | -0.249910 | -0.288560 | -0.141640 | -0.141510 |

Table S15: Continued

| bond length | HF | phRPA@HF | ppRPA@HF | MR-ppRPA@HF | CCSD |
|---|---|---|---|---|---|
| 1.1 | -0.319130 | -0.231640 | -0.269770 | -0.125300 | -0.125180 |
| 1.2 | -0.299070 | -0.212370 | -0.249950 | -0.108410 | -0.108300 |
| 1.3 | -0.278890 | -0.193110 | -0.230080 | -0.092040 | -0.091930 |
| 1.4 | -0.259150 | -0.174440 | -0.210720 | -0.076820 | -0.076710 |
| 1.5 | -0.240150 | -0.156700 | -0.192190 | -0.063080 | -0.062980 |
| 1.6 | -0.222050 | -0.140070 | -0.174680 | -0.051010 | -0.050900 |
| 1.7 | -0.204960 | -0.124650 | -0.158280 | -0.040660 | -0.040550 |
| 1.8 | -0.188890 | -0.110470 | -0.143020 | -0.031990 | -0.031880 |
| 1.9 | -0.173870 | -0.097530 | -0.128920 | -0.024880 | -0.024760 |
| 2.0 | -0.159860 | -0.085790 | -0.115930 | -0.019160 | -0.019030 |
| 2.1 | -0.146820 | -0.075180 | -0.104000 | -0.014630 | -0.014500 |
| 2.2 | -0.134700 | -0.065630 | -0.093090 | -0.011090 | -0.010960 |
| 2.3 | -0.123440 | -0.057050 | -0.083110 | -0.008360 | -0.008230 |
| 2.4 | -0.112990 | -0.049380 | -0.074020 | -0.006280 | -0.006150 |
| 2.5 | -0.103290 | -0.042530 | -0.065750 | -0.004690 | -0.004570 |
| 2.6 | -0.094290 | -0.036440 | -0.058230 | -0.003500 | -0.003380 |
| 2.7 | -0.085940 | -0.031030 | -0.051420 | -0.002600 | -0.002500 |
| 2.8 | -0.078210 | -0.026260 | -0.045260 | -0.001940 | -0.001840 |
| 2.9 | -0.071040 | -0.022060 | -0.039700 | -0.001440 | -0.001350 |
| 3.0 | -0.064400 | -0.018390 | -0.034700 | -0.001070 | -0.000990 |
| 3.1 | -0.058260 | -0.015180 | -0.030200 | -0.000790 | -0.000730 |
| 3.2 | -0.052570 | -0.012400 | -0.026180 | -0.000590 | -0.000530 |
| 3.3 | -0.047310 | -0.010000 | -0.022590 | -0.000440 | -0.000390 |
| 3.4 | -0.042440 | -0.007950 | -0.019390 | -0.000320 | -0.000290 |

Table S15: Continued

| bond length | HF | phRPA@HF | ppRPA@HF | MR-ppRPA@HF | CCSD |
|---|---|---|---|---|---|
| 3.5 | -0.037950 | -0.006200 | -0.016550 | -0.000240 | -0.000210 |
| 3.6 | -0.033800 | -0.004730 | -0.014040 | -0.000180 | -0.000160 |
| 3.7 | -0.029970 | -0.003500 | -0.011830 | -0.000130 | -0.000110 |
| 3.8 | -0.026430 | -0.002480 | -0.009890 | -0.000100 | -0.000080 |
| 3.9 | -0.023170 | -0.001660 | -0.008190 | -0.000070 | -0.000060 |
| 4.0 | -0.020150 | -0.001000 | -0.006710 | -0.000050 | -0.000050 |
| 4.1 | -0.017370 | -0.000490 | -0.005440 | -0.000040 | -0.000030 |
| 4.2 | -0.014800 | -0.000110 | -0.004330 | -0.000030 | -0.000030 |
| 4.3 | -0.012430 | 0.000160 | -0.003390 | -0.000020 | -0.000020 |
| 4.4 | -0.010240 | 0.000340 | -0.002590 | -0.000020 | -0.000010 |
| 4.5 | -0.008200 | 0.000430 | -0.001920 | -0.000010 | -0.000010 |
| 4.6 | -0.006320 | 0.000450 | -0.001360 | -0.000010 | -0.000010 |
| 4.7 | -0.004560 | 0.000410 | -0.000890 | 0.000000 | 0.000000 |
| 4.8 | -0.002940 | 0.000320 | -0.000520 | 0.000000 | 0.000000 |
| 4.9 | -0.001420 | 0.000180 | -0.000230 | 0.000000 | 0.000000 |
| 5.0 | 0.000000 | 0.000000 | 0.000000 | 0.000000 | 0.000000 |

Table S16: Total energies of $Ar_2$ obtained from HF, phRPA@HF, ppRPA@HF and CCSD(T). The cc-pVDZ basis set was used. All bond lengths are in angstrom and energy values are in Hartree.

| bond length | HF | phRPA@HF | ppRPA@HF | CCSD(T) |
|---|---|---|---|---|
| 3.0 | 0.006100 | 0.005030 | 0.004890 | 0.004890 |
| 3.1 | 0.004180 | 0.003320 | 0.003210 | 0.003220 |
| 3.2 | 0.002840 | 0.002160 | 0.002070 | 0.002070 |

Table S16: Continued

| bond length | HF | phRPA@HF | ppRPA@HF | CCSD(T) |
|---|---|---|---|---|
| 3.3 | 0.001910 | 0.001370 | 0.001290 | 0.001300 |
| 3.4 | 0.001270 | 0.000840 | 0.000780 | 0.000790 |
| 3.5 | 0.000830 | 0.000490 | 0.000440 | 0.000440 |
| 3.6 | 0.000530 | 0.000260 | 0.000210 | 0.000220 |
| 3.7 | 0.000330 | 0.000120 | 0.000070 | 0.000080 |
| 3.8 | 0.000190 | 0.000030 | -0.000010 | 0.000000 |
| 3.9 | 0.000110 | -0.000030 | -0.000060 | -0.000050 |
| 4.0 | 0.000050 | -0.000050 | -0.000080 | -0.000080 |
| 4.1 | 0.000020 | -0.000070 | -0.000090 | -0.000080 |
| 4.2 | 0.000000 | -0.000070 | -0.000090 | -0.000080 |
| 4.3 | -0.000010 | -0.000060 | -0.000080 | -0.000080 |
| 4.4 | -0.000010 | -0.000060 | -0.000070 | -0.000070 |
| 4.5 | -0.000010 | -0.000050 | -0.000060 | -0.000060 |
| 4.6 | -0.000010 | -0.000040 | -0.000050 | -0.000050 |
| 4.7 | -0.000010 | -0.000030 | -0.000040 | -0.000040 |
| 4.8 | -0.000010 | -0.000030 | -0.000040 | -0.000030 |
| 4.9 | 0.000000 | -0.000020 | -0.000030 | -0.000030 |
| 5.0 | 0.000000 | -0.000020 | -0.000020 | -0.000020 |
| 5.1 | 0.000000 | -0.000010 | -0.000020 | -0.000020 |
| 5.2 | 0.000000 | -0.000010 | -0.000020 | -0.000010 |
| 5.3 | 0.000000 | -0.000010 | -0.000010 | -0.000010 |
| 5.4 | 0.000000 | -0.000010 | -0.000010 | -0.000010 |
| 5.5 | 0.000000 | 0.000000 | -0.000010 | -0.000010 |
| 5.6 | 0.000000 | 0.000000 | -0.000010 | 0.000000 |

Table S16: Continued

| bond length | HF | phRPA@HF | ppRPA@HF | CCSD(T) |
|---|---|---|---|---|
| 5.7 | 0.000000 | 0.000000 | 0.000000 | 0.000000 |
| 5.8 | 0.000000 | 0.000000 | 0.000000 | 0.000000 |
| 5.9 | 0.000000 | 0.000000 | 0.000000 | 0.000000 |
| 6.0 | 0.000000 | 0.000000 | 0.000000 | 0.000000 |

# References


(S1) Bernard, Y. A.; Shao, Y.; Krylov, A. I. General Formulation of Spin-Flip Time-Dependent Density Functional Theory Using Non-Collinear Kernels: Theory, Implementation, and Benchmarks. *J. Chem. Phys.* **2012**, *136*, 204103.

(S2) Ess, D. H.; Johnson, E. R.; Hu, X.; Yang, W. Singlet-Triplet Energy Gaps for Diradicals from Fractional-Spin Density-Functional Theory. *J. Phys. Chem. A* **2011**, *115*, 76–83.

(S3) Yang, Y.; Peng, D.; Davidson, E. R.; Yang, W. Singlet–Triplet Energy Gaps for Diradicals from Particle–Particle Random Phase Approximation. *J. Phys. Chem. A* **2015**, *119*, 4923–4932.

(S4) Huber, K. P.; Herzberg, G. *Molecular Spectra and Molecular Structure: IV. Constants of Diatomic Molecules*; Springer US: Boston, MA, 1979; pp 8–689.

(S5) Yang, Y.; Davidson, E. R.; Yang, W. Nature of Ground and Electronic Excited States of Higher Acenes. *Proc. Natl. Acad. Sci.* **2016**, *113*, E5098–E5107.

(S6) Yu, J.; Li, J.; Zhu, T.; Yang, W. Accurate and Efficient Prediction of Double Exci-

tation Energies Using the Particle–Particle Random Phase Approximation. *J. Chem. Phys.* **2025**, *162*, 094101.

(S7) Kossoski, F.; Boggio-Pasqua, M.; Loos, P.-F.; Jacquemin, D. Reference Energies for Double Excitations: Improvement and Extension. *J. Chem. Theory Comput.* **2024**, *20*, 5655–5678.

(S8) Li, J.; Jin, Y.; Su, N. Q.; Yang, W. Combining Localized Orbital Scaling Correction and Bethe–Salpeter Equation for Accurate Excitation Energies. *J. Chem. Phys.* **2022**, *156*, 154101.

(S9) Stein, T.; Kronik, L.; Baer, R. Reliable Prediction of Charge Transfer Excitations in Molecular Complexes Using Time-Dependent Density Functional Theory. *J. Am. Chem. Soc.* **2009**, *131*, 2818–2820.

(S10) Li, J.; Golze, D.; Yang, W. Combining Renormalized Singles GW Methods with the Bethe–Salpeter Equation for Accurate Neutral Excitation Energies. *J. Chem. Theory Comput.* **2022**, *18*, 6637–6645.

(S11) Xu, X.; Yang, K. R.; Truhlar, D. G. Testing Noncollinear Spin-Flip, Collinear Spin-Flip, and Conventional Time-Dependent Density Functional Theory for Predicting Electronic Excitation Energies of Closed-Shell Atoms. *J. Chem. Theory Comput.* **2014**, *10*, 2070–2084.

(S12) Yang, Y.; Peng, D.; Lu, J.; Yang, W. Excitation Energies from Particle-Particle Random Phase Approximation: Davidson Algorithm and Benchmark Studies. *J. Chem. Phys.* **2014**, *141*, 124104.

(S13) Silva-Junior, M. R.; Schreiber, M.; Sauer, S. P. A.; Thiel, W. Benchmarks for Electronically Excited States: Time-dependent Density Functional Theory and Density Functional Theory Based Multireference Configuration Interaction. *J. Chem. Phys.* **2008**, *129*, 104103.

(S14) Li, J.; Jin, Y.; Yu, J.; Yang, W.; Zhu, T. Accurate Excitation Energies of Point Defects from Fast Particle–Particle Random Phase Approximation Calculations. *J. Phys. Chem. Lett.* **2024**, *15*, 2757–2764.

(S15) Li, J.; Jin, Y.; Yu, J.; Yang, W.; Zhu, T. Particle–Particle Random Phase Approximation for Predicting Correlated Excited States of Point Defects. *J. Chem. Theory Comput.* **2024**, *20*, 7979–7989.

(S16) Davies, G.; Hamer, M. F.; Price, W. C. Optical Studies of the 1.945 eV Vibronic Band in Diamond. *Proc. R. Soc. Lond. Math. Phys. Sci.* **1997**, *348*, 285–298.

(S17) Haldar, S.; Mitra, A.; Hermes, M. R.; Gagliardi, L. Local Excitations of a Charged Nitrogen Vacancy in Diamond with Multireference Density Matrix Embedding Theory. *J. Phys. Chem. Lett.* **2023**, *14*, 4273–4280.

(S18) Lannoo, M.; Stoneham, A. M. The Optical Absorption of the Neutral Vacancy in Diamond. *Journal of Physics and Chemistry of Solids* **1968**, *29*, 1987–2000.

(S19) Chen, Y.; Williams, R. T.; Sibley, W. A. Defect Cluster Centers in MgO. *Phys. Rev.* **1969**, *182*, 960–964.

(S20) Kappers, L. A.; Kroes, R. L.; Hensley, E. B. ${F}^{+}$ and ${F}^{\ensuremath{'}}$ Centers in Magnesium Oxide. *Phys. Rev. B* **1970**, *1*, 4151–4157.

(S21) Zheng, J.; Zhao, Y.; Truhlar, D. G. Representative Benchmark Suites for Barrier Heights of Diverse Reaction Types and Assessment of Electronic Structure Methods for Thermochemical Kinetics. *J. Chem. Theory Comput.* **2007**, *3*, 569–582.

(S22) Yang, Y.; van Aggelen, H.; Steinmann, S. N.; Peng, D.; Yang, W. Benchmark Tests and Spin Adaptation for the Particle-Particle Random Phase Approximation. *J. Chem. Phys.* **2013**, *139*, 174110.

(S23) van Aggelen, H.; Yang, Y.; Yang, W. Exchange-Correlation Energy from Pairing Matrix Fluctuation and the Particle-Particle Random Phase Approximation. *J. Chem. Phys.* **2014**, *140*, 18A511.
